# Supplementary material for: Insight of the thermal conductivity of $\epsilon-$iron at Earth's core conditions from the newly developed direct $ab~initio$ methodology
Source: arXiv:1808.10860 source file (2018-08-31)
Supplement: Supplementary file 1 [file SI.pdf]

Supplementary Materials for

# Insight of the thermal conductivity of ε-iron at Earth's core conditions from the newly developed direct *ab initio* methodology


Sheng-Ying Yue[1,2,*] and Ming Hu[1,3,4,†]

[1]*Aachen Institute for Advanced Study in Computational Engineering Science (AICES), RWTH Aachen University, 52062 Aachen, Germany*

[2]*Department of Mechanical Engineering, University of California, Santa Barbara, CA 93106, USA*

[3]*Institute of Mineral Engineering, Division of Materials Science and Engineering, Faculty of Georesources and Materials Engineering, RWTH Aachen University, 52064 Aachen, Germany*

[4]*College of Engineering and Computing, University of South Carolina, SC 29208, USA*

Author to whom all correspondence should be addressed. *E-Mail: sheng.ying.yue@rwth-aachen.de (S.-Y.Y.) and †E-Mail: hu@sc.edu (M.H.).

## 1. NEAIMD simulation setup

All AIMD simulations are performed using the DFT method implemented in VASP [1, 2]. The Perdew-Burke-Ernzerhof parameterization of the generalized gradient approximation (GGA) is used for the exchange-correlated functional [3], and the projector-augmented wave method is applied to model the core electrons [4, 5].

The $3p^6 4s^1 3d^7$ valence electronic configuration is adopted, and the core radii is 1.16 Å [6-8]. Single particle orbitals were expanded in plane-waves with a cutoff of 380 eV. Electronic levels were occupied according to Fermi-Dirac statistics, with electronic temperature corresponding to the temperature of the system.

For the energy cut-off, we use the default value in the pseudopotential file. We first relax the system with the $NpT$-ensemble (constant number of particles, pressure, and temperature) at room temperature to obtain the lattice constants of the metals at a finite temperature. We then apply the resulting lattice constants to construct the initial structures for subsequent NEAIMD simulations. The NEAIMD simulations are performed using a modified version of the VASP code [9, 10] with the $NVE$ ensemble (constant volume and no thermostat). An efficient extrapolation of the charge density was used to speed up the NEAIMD simulations [11] by sampling the Brillouin zone (BZ) with the Γ point only. The temperature was controlled with Andersen thermostat [12] and the time step was set as 1 fs. We run simulations for typically 8-10 ps, from which we discarded the first around 0.3 ps to allow the system to reach equilibrium.

We apply a fixed boundary condition along the direction of the heat flux and periodic boundary conditions in the two lateral directions (perpendicular to the direction of the heat flux) of the simulation model (see Fig. 1(a) in the main article) [10]. To avoid self-interaction between periodic images of the simulation cell, in the direction of the heat flux, we add a vacuum layer with a thickness exceeding 5 Å on the external sides of the fixed atom layers. The total distance between the periodic images of the simulation model exceeds 10 Å in real space [10]. The layers next to the fixed layers are the heat-source and heat-sink. A constant atomic heat flux is imposed by applying the Müller-Plathe algorithm [13]. The coldest atom in the hot region and the hottest atom in the cold region are selected, and their kinetic energies (atomic velocities) are exchanged every 40 fs with a 1-fs time step. This operation induces a steady heat-energy-flux in the system and a corresponding temperature gradient (∇T) after running for a sufficiently long time. The energy-exchange time interval is used to control the temperature gradient's magnitude. The linear portion of the temperature gradient lies between the heat baths. With sufficient simulation time, we can establish a steady ∇T in metals. By linear fitting the statistically averaged temperatures of each atom layer, we obtain ∇T, which is used to calculate the final electronic thermal conductivity ($\kappa_{el}$) and phonon thermal conductivity ($\kappa_{ph}$) [10].

For ϵ-iron at Earth's core conditions, the size of simulation model is 4 × 4 × 8 conventional cells (16 atom layers along the heat flux direction). To study size effects, we examine models with a length of 14, 18, 22 atom layers for ϵ-iron, 4 × 4 × (7, 9, 11) conventional cells, we also investigate the size effect of the cross-section using a model with 2 × 4 × 8 conventional cells. The basic information for all NEAIMD simulations is presented in Table 1. Additionally, a short animation of the NEAIMD of ϵ-iron is given to show the real simulation process.

Table 1: Details of NEAIMD simulation of ϵ-iron

| System | System length (Å) | Cross-sectional area ($S$, Å$^2$) | Atom number | Total simulation time (t, ps) | Average temperature (T, K) | Average pressure (P, GPa) |
|---|---|---|---|---|---|---|
| ϵ-iron | 29.4072 | 59.6880 | 256 | 8 | 3740.81 | 136.44 |
| | 29.4072 | 59.6880 | | 8 | 3915.86 | 136.74 |
| | 28.9842 | 56.1212 | | 8 | 5289.47 | 316.20 |
| | 28.9130 | 55.8461 | | 8 | 5904.63 | 323.67 |
| | 28.8917 | 55.7637 | | 8 | 5543.93 | 327.39 |
| | 28.8953 | 55.7774 | | 8 | 5835.26 | 327.47 |
| | 28.8953 | 55.7774 | | 8 | 6377.60 | 330.68 |
| | 28.7708 | 55.2979 | | 8 | 5435.12 | 360.71 |
| | 28.7708 | 55.2979 | | 8 | 5661.80 | 362.00 |
| | 28.7708 | 55.2979 | | 8 | 6238.93 | 365.32 |
| | 25.7375 | 55.7774 | 224 | 8 | 6291.28 | 331.21 |
| | 32.1612 | 56.1487 | 288 | 6 | 6382.81 | 330.90 |
| | 35.3303 | 56.1487 | 320 | 4 | 6376.92 | 331.79 |

## 2. Calculation of thermal conductivity κ of ϵ-Fe from NEAIMD

### 2.1 Heat flux via free electrons $\vec{J}_{el}$

The EP expression used in VASP is defined as

$$U = \int U(r) \cdot \rho_{test} \cdot (|r - R|) d^3 r, \quad (1)$$

where the test charge $\rho_{test}$ is norm 1. From this formula, we can see that the EP $U$ is a function of ion position $R$. We apply the RMS method [14] to calculate the average effective amplitude of EPO ($\overline{U}_{EPO}$)

$$\overline{U}_{EPO}(l) = \frac{1}{N_{al}} \sum_{j=1}^{N_{al}} \sqrt{\frac{1}{n_{steps}} \sum_{i=1}^{n_{steps}} (U_j(t_i) - \overline{U}_j)^2}, \quad (2)$$

where $l$ is the index of the atom layers, $N_{al}$ is the total number of atoms per layer, $n_{steps}$ is the total number of simulation steps, $U_j(t_i)$ is the EP displacement of ion core $j$ at $i$ fs, and $\overline{U}_j$ is the average value of $U_j(t_i)$ for atom $j$ in layer $l$. $\overline{U}_{EPO}(l)$ represents the intensity of the local EPO. Thus, the energy provided by EPO in each layer $E_{EPO}(l)$ can be written as

$$E_{EPO}(l) = 2 \cdot \overline{U}_{EPO}(l) \cdot n(e) \cdot e \quad (3)$$

$n(e)$ is the number of valance electrons per atom layer. Here for the ϵ-Fe under the Earth's core conditions, the $3p^6 4s^1 3d^7$ valence electronic configuration is adopted. Now, we have calculate the average effective EPO amplitude $\overline{U}_{EPO}(l)$ and effective EPO energy $E_{EPO}(l)$. Then, we can obtain the total effective energy provided by EPO during simulation time $t$ as

$$E_{EPO}(l, t) = 2 \cdot \overline{U}_{EPO}(l) \cdot n(e) \cdot e \cdot n_{steps}, \quad (4)$$

where $n_{steps}$ is the total number of time steps during the simulation time $t$. When the system reaches a quasi-equilibrium state, we can infer that the thermal energy of thermally excited electrons is exchanged between two adjacent atom layers [10]. As illustrated in Fig. S1, we take half of the difference of the thermal kinetic energy exchange between the two layers as $\vec{J}_{el}$ (because of the isotropy of the free electron model)

$$\vec{J}_{el} = -\frac{1}{2}\frac{n(e)\cdot e}{S\cdot t}\frac{\partial\left[2\cdot \bar{U}_{EPO}(l)\cdot n_{steps}\right]}{\partial N_l} = -\frac{n(e)\cdot e\cdot n_{steps}}{S\cdot t}\frac{\partial \bar{U}_{EPO}(l)}{\partial N_l}, \quad (5)$$

where $S$ is the cross-sectional area, $n(e)$ is the number of free electrons per atom layer, $e$ is the unit charge of a single electron, and $\frac{\partial \bar{U}_{EPO}(l)}{\partial N_l}$ is the gradient of the average effective EPO amplitude value by linear fitting of $\bar{U}_{EPO}(l)$ with respect to the index number of atom layers ($N_l$), as shown in Fig. S2.

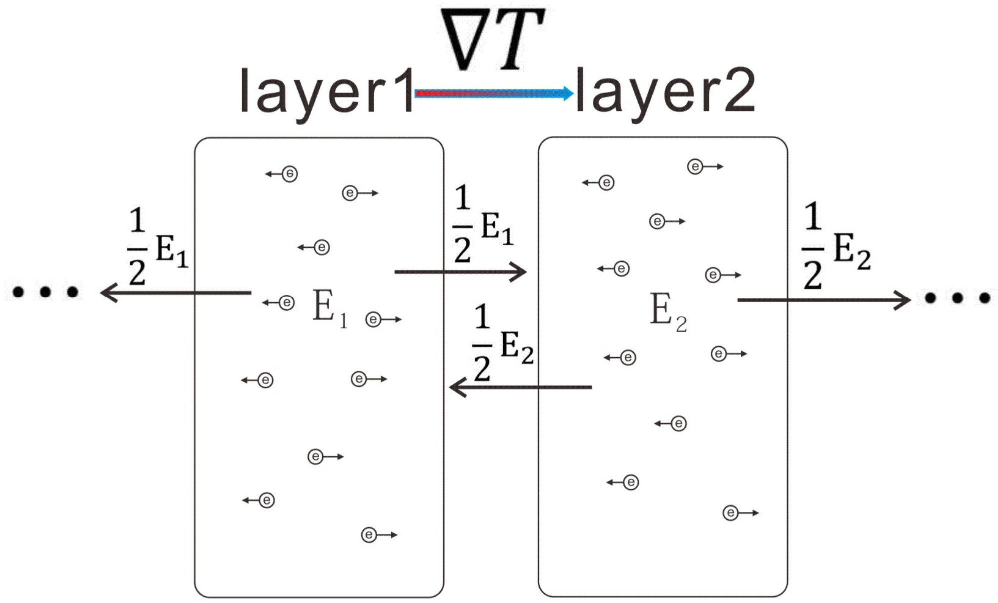


Fig. S1: Schematic of the exchange of thermal excited electrons' thermal energy between two adjacent atom layers. $E_1$ and $E_2$ are the thermal energies carried by thermally excited electrons in layer1 and layer2, respectively.

## 2.2 Electronic thermal conductivity ($\kappa_{el}$)

From Fourier's Law of heat conduction, the electronic thermal conductivity ($\kappa_{el}$) can be written as

$$\kappa_{el} = -J_{el}/\nabla T. \quad (6)$$

Combining Equation (6) with Equation (5), we have

$$\kappa_{el} = \frac{n(e) \cdot e \cdot n_{steps}}{S \cdot t \cdot \nabla T} \frac{\partial \bar{U}_{EPO}(l)}{\partial N_l}. \tag{7}$$

Based on Eq. (7), we calculate the $\kappa_{el}$ of ϵ-Fe at ICB and CMB conditions. We run multiple NEAIMD simulations for each system with different $T$ to examine the temperature dependent thermal conductivity of metals. All the simulation results are reported in Table 2.

## 2.3 Results of the EPO in space

We present the distribution of the effective amplitude of EPO in space rather than that of the thermal kinetic energy of thermally excited electrons, in Fig. S2.

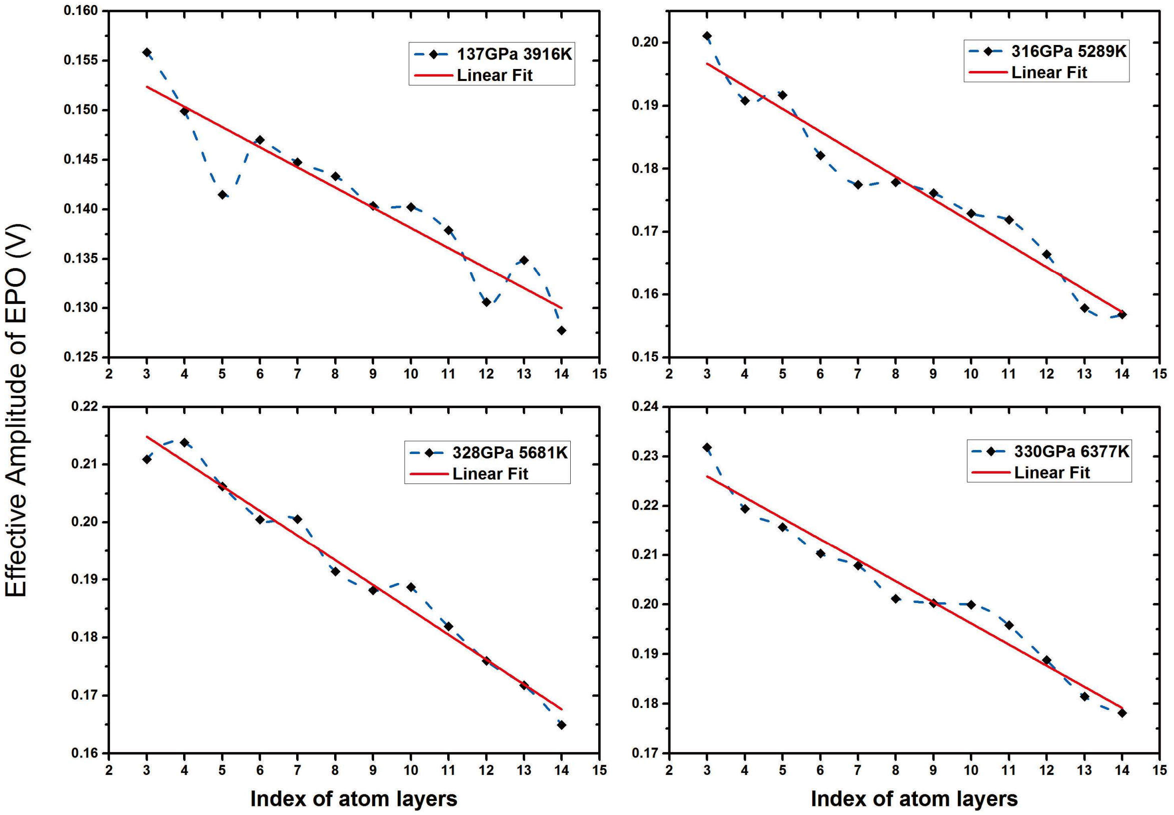


Fig. S2: Effective amplitudes of the EPO along the direction of the heat flux in ϵ-Fe with different conditions in CMB and ICB. Via linear fitting, we can obtain $\frac{\partial \bar{U}_{EPO}(l)}{\partial N_l}$, which is used to calculate electronic heat flux.

Fig. S2 shows that in ϵ-Fe, higher temperatures increase the strength of EPO. We also note that a non-linear phenomenon of $\bar{U}_{EPO}(l)$ occurs in some cases, such as at 137 GPa and 3916 K. This phenomenon will cause significant errors in the final electronic thermal conductivity ($\kappa_{el}$).

## 2.4 The non-linear effect analysis

To elucidate the reason for this non-linear phenomenon, we plot the temperature profiles of different metals in Fig. S3. We can see that the degree of the non-linear temperature distributions of ϵ-Fe at 137 GPa and 3916 K is larger than others. The non-linear temperature distribution may be responsible for the non-linear distribution of $\overline{U}_{EPO}(l)$.

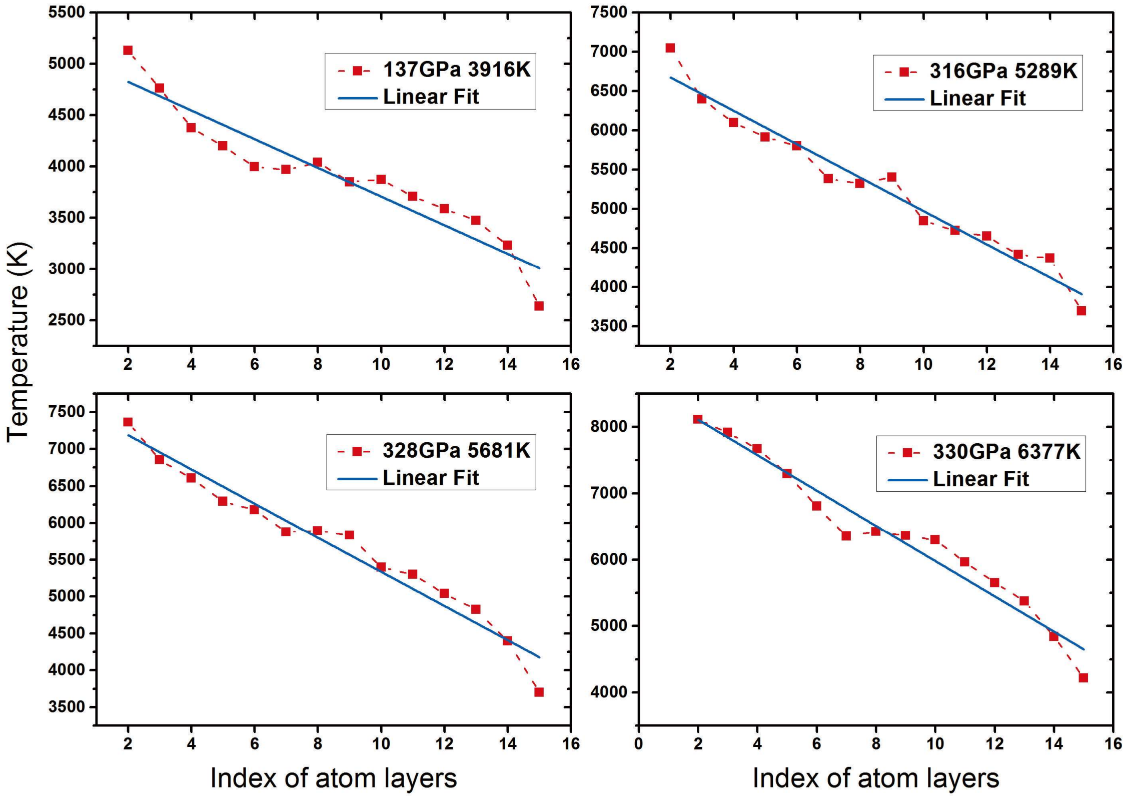


Fig. S3: Temperature profiles from NEAIMD simulations of ϵ-Fe with different conditions in CMB and ICB. The dashed line is the linear fit of the temperature profile, i.e., the temperature gradient ($\nabla T$).

We also attempt to examine the non-linear effect by increasing the model size. Fig. S4 and Fig. S5. present the NEAIMD temperature profile and the EPO distributions in space of different ϵ-Fe lengths at ~330 GPa and ~6300 K. Based on these results, we recognize that the simulation size will indeed affect the non-linear EPO phenomenon in ϵ-iron. And these non-linear effects will be directly reflected in error-bar of $\kappa_{el}$.

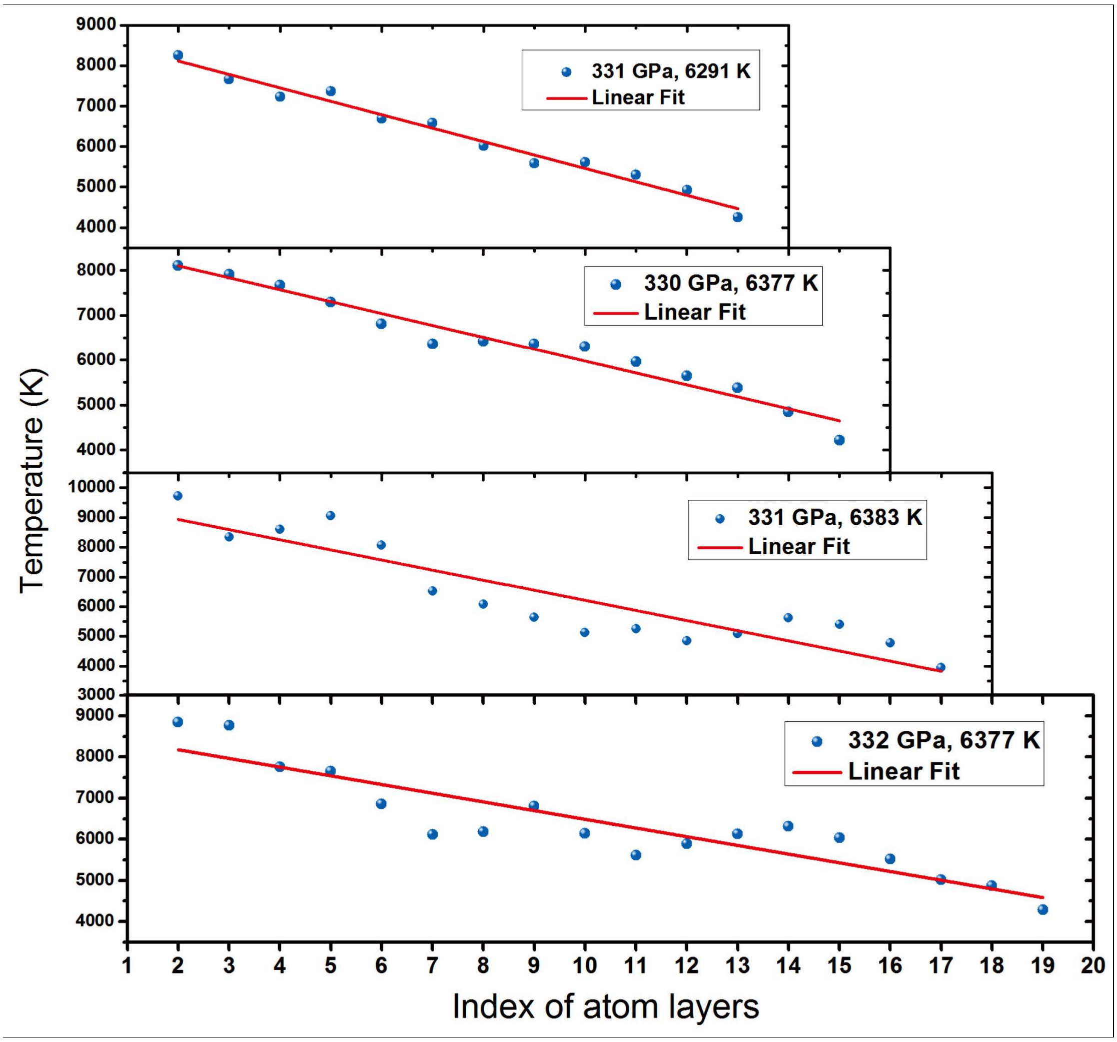


Fig. S4: Distributions of the temperature profile for different lengths of ϵ-Fe with different conditions in CMB and ICB.

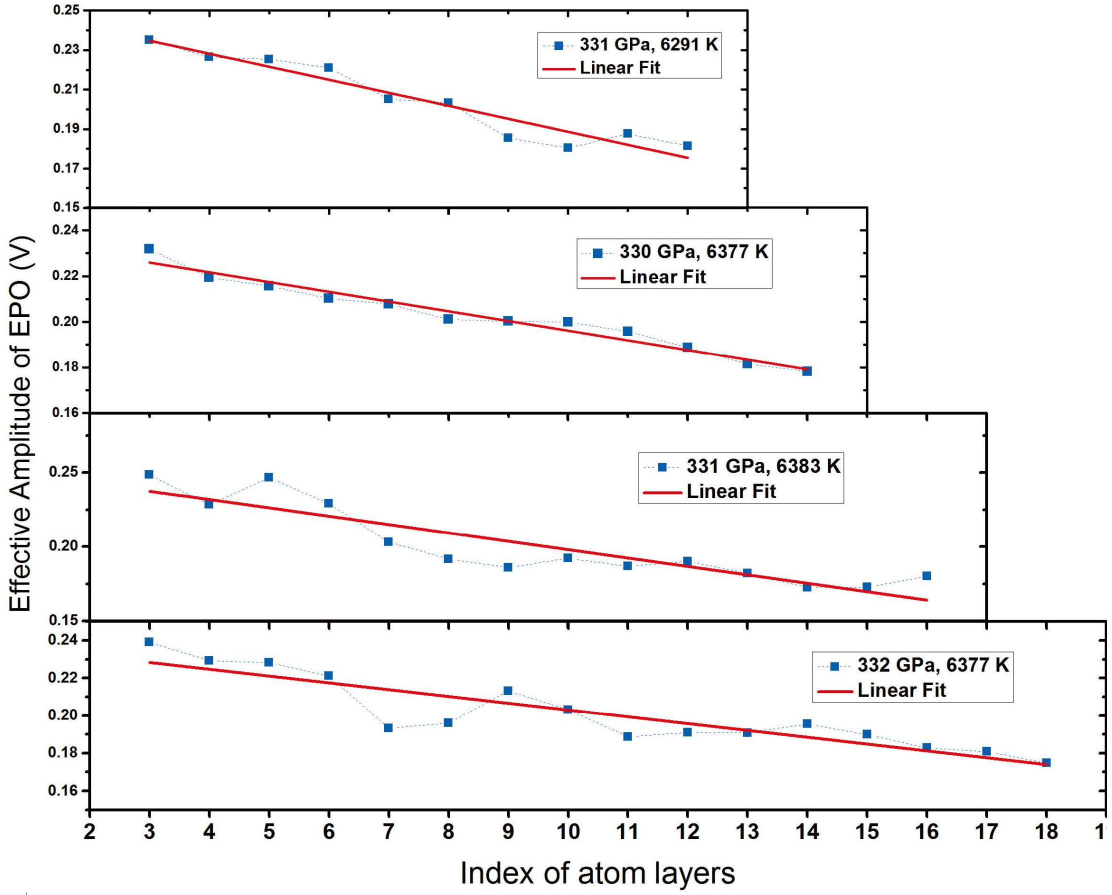


Fig. S5: Distributions of the effective amplitude of EPO along $\nabla T$ for different lengths of ϵ-Fe with different conditions in CMB and ICB.

## 2.5 Phonon thermal conductivity ($\kappa_{ph}$)

As we employ the Müller-Plathe algorithm to establish a stable temperature gradient along the heat transfer direction [13], we can also obtain the atomic kinetic energy flux $J_{ph}$. See the representative NEAIMD simulating case in Fig.S6. We calculated the phonon thermal conductivity ($\kappa_{ph}$) simultaneously from Fourier's Law:

$$\kappa_{ph} = -J_{ph}/\nabla T. \tag{8}$$

The results are also reported in Table 2. By summing $\kappa_{el}$ and $\kappa_{ph}$, we obtain the total $\kappa$ of metals from parameter free NEAIMD simulations.

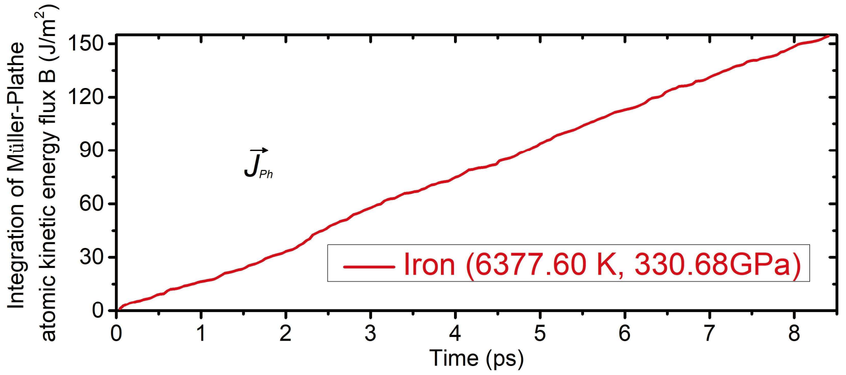


Fig.S6: The corresponding integration of the atomic kinetic energy flux with time.

Table 2: Electronic thermal conductivity $\kappa_{el}$ and phonon thermal conductivity $\kappa_{ph}$ from NEAIMD.

| Average pressure (P, GPa) | Average temp. (T, K) | Temperature gradient $\nabla T$ (K/Å) | Electronic thermal conductivity $\kappa_{el}$ (W/mK) | Phonon thermal conductivity $\kappa_{ph}$ (W/mK) | Total thermal conductivity $\kappa$ (W/mK) | Total error bar of $\kappa_{el}$ (W/mK) |
|---|---|---|---|---|---|---|
| **136.44** | 3740.81 | -82.97 | 198.09 | 10.67 | 208.76 | 23.90 |
| **136.74** | 3915.86 | -66.63 | 183.77 | 13.47 | 197.24 | 14.55 |
| **316.20** | 5289.47 | -115.49 | 198.74 | 12.95 | 211.69 | 9.00 |
| **323.67** | 5904.63 | -140.40 | 167.23 | 11.43 | 178.66 | 11.43 |
| **327.39** | 5543.93 | -136.99 | 182.40 | 11.10 | 193.5 | 8.88 |
| **327.47** | 5835.26 | -129.14 | 173.71 | 11.57 | 185.28 | 9.69 |
| **330.68** | 6377.60 | -153.16 | 178.62 | 11.89 | 190.51 | 8.50 |
| **360.71** | 5435.12 | -111.05 | 197.95 | 14.78 | 212.73 | 17.20 |
| **362.00** | 5661.80 | -114.92 | 201.05 | 12.85 | 213.9 | 13.36 |
| **365.32** | 6238.93 | -136.31 | 188.98 | 13.26 | 202.24 | 10.99 |
| **331.21** | 6291.28 | -191.77 | 221.00 | 8.78 | 229.78 | 10.52 |
| **330.90** | 6382.81 | -198.08 | 182.43 | 7.17 | 189.6 | 8.68 |
| **331.79** | 6376.92 | -116.66 | 198.64 | 15.97 | 214.61 | 9.45 |

## 2.6 The examination of the thermal conductivity of b.c.c iron

To examine the correction of our strategy for adopting the pseudo-potential for iron, here, we also apply the NEAIMD-EPO method to simulate the b.c.c iron at ambient condition. The results are presented in Table 3.

Table 3: thermal conductivity ($\kappa_{el} + \kappa_{ph}$) of b.c.c iron at ambient condition from NEAIMD-EPO method.

| Case-ID(b.c.c) | Temperature (K) | Pressure(GPa) | Time(ps) | Length (nm) | $\kappa$ (W/mK) |
|---|---|---|---|---|---|
| 1 | 290.80 | -3.05 | 2.12 | 2.5305 | 87.24±9.99 |
| 2 | 290.80 | -3.05 | 2.13 | 2.5305 | 87.41±10.01 |
| 3 | 394.05 | -2.84 | 2.13 | 2.5305 | 78.86±9.03 |
| 4 | 292.28 | -1.22 | 7.62 | 3.1001 | 85.64±9.81 |
| 5 | 296.12 | -3.46 | 4.72 | 2.5305 | 83.68±9.58 |
| Experiment | 300 | 0.0001 | | | 80.2 |

### 2.7 Size effects of lattice thermal conductivity $\kappa_{ph}$ from NEAIMD

It is well known that, in lattice dynamics each vibrational mode (phonon) has a specific wave-length. In view of this, finite size effects are inevitable in non-equilibrium molecular dynamics (NEMD) simulations of lattice thermal conductivity of most systems, where phonons are truncated due to the limited model length [15]. We recognize that there exist the size effects limitation of $\kappa_{ph}$ in our NEAIMD simulations. Here we present the size-effect of the lattice thermal conductivity of our NEAIMD in Table 4.

Table 4. $\kappa_{ph}$ of ϵ-iron at earth's core conditions from NEAIMD.

| Case-ID | Temperature (K) | Pressure (GPa) | Time(ps) | Length (nm) | $\kappa_{ph}$ (W/mK) |
|---|---|---|---|---|---|
| 1 | 6291.3 | 331.2 | 4 | 2.57375 | 8.78 |
| 2 | 6382.8 | 330.9 | 4 | 3.21612 | 10.29 |
| 3 | 6376.9 | 331.7 | 4 | 3.53303 | 11.96 |

From Table 4. We can see the size-effect of $\kappa_{ph}$ in NEAIMD simulation. The size-effect limitation will lead to underestimate the $\kappa_{ph}$ here. However, we can clearly see that the $\kappa_{el}$ dominates the thermal transport in ϵ-iron at Earth's core conditions. Unlike $\kappa_{ph}$, from our NEAIMD simulations results, we do not observe a clear size effect for $\kappa_{el}$ [10]. In addition, the error-bar of the $\kappa_{ph}$ in NEAIMD simulation mainly originates from the fitting the temperature gradient $\nabla T$, we calculated the error-bars of the $\kappa_{ph}$ for the ϵ-iron at Earth's core conditions and present the data in the main manuscript TABLE.1.

### 2.8 $\kappa_{ph}$ from the Boltzmann transport equation (BTE)

For comparing the lattice thermal conductivity from NEAIMD with the results of other method, we calculate $\kappa_{ph}$ of ϵ-iron at 330.68 GPa and temperature ranging from 6350 K to 6400 K by solving the phonon BTE, with force constants extracted from first-principles calculations. The phonon BTE model does not suffer from finite size effects. We employ the first-principle software package VASP [1,2] to calculate the second-order (harmonic) and third-order (anharmonic) force constants based on the finite displacement difference method [16, 17], and then use the ShengBTE package [17] to obtain $\kappa_{ph}$ by iteratively solving the BTE of phonons. The convergences of $\kappa_{ph}$ with respect to the $k$-grid size ($N \times N \times N$) in our calculations are fully examined and the parameter $N = 20$ is taken to evaluate the converged $\kappa_{ph}$. The convergences of $\kappa_{ph}$ with respect to the force cut-off distance are also examined and we took the distance of the fifth-order adjacent neighbor atoms as the force cut-off. The energy of plane-wave cutoff is adopted the value of 1.5 times of the default value in VASP pseudo-potential files.

In Fig.S7, Fig.S8 and Fig.S9, we present the phonon dispersion, phonon group velocities and phonon lifetime of the ϵ-iron at 330.68 GPa, respectively. All these physical quantities are from the phonon BTE calculations. Because that the fourth- and higher order anharmonicity will become very important at high temperature [18], the phonon BTE method should overestimate the $\kappa_{ph}$. We present the $\kappa_{ph}$ results from the BTE method in Fig. S10. From Fig.S10, we can learn that the $\kappa_{ph}$ of ϵ-iron at 330.68 GPa, 6350 K~6400 K is around the 28 W/(mK), which is much larger than our NEAIMD result $12 \pm 3\ \mathrm{W/(mK)}$. Although the NEAIMD method will underestimate the $\kappa_{ph}$ value because of the size-effect limitation, the BTE method should be overestimate the $\kappa_{ph}$ at

extreme high temperature condition because it only considers the third-order phonon anharmonicity, i.e. without fourth- and higher-order phonon anharmonicity which are important at high temperatures [18].

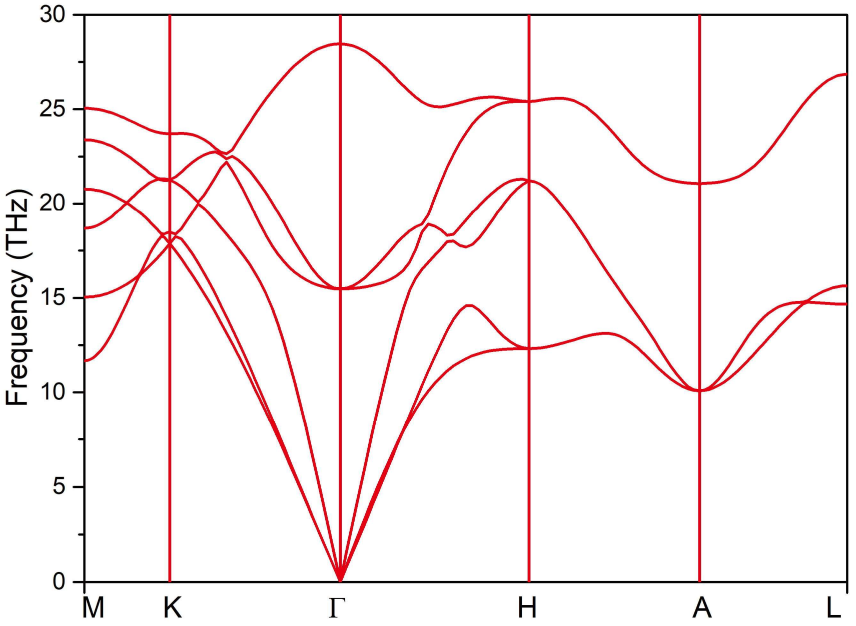


Fig.S7: The phonon dispersion of ε-iron at 330.68 GPa.

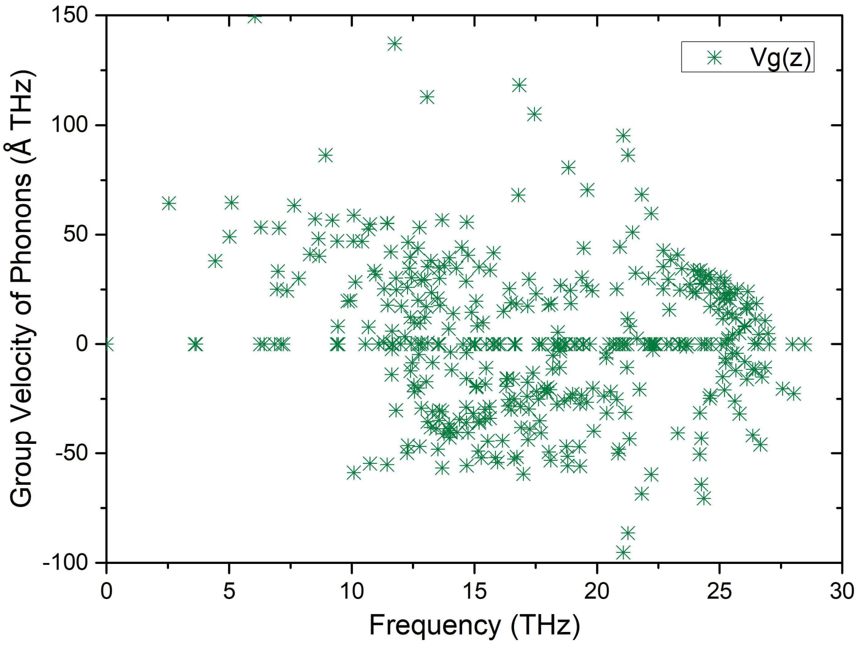


Fig.S8: The phonon group velocities (along heat flux direction z) of ε-iron at 330.68 GPa.

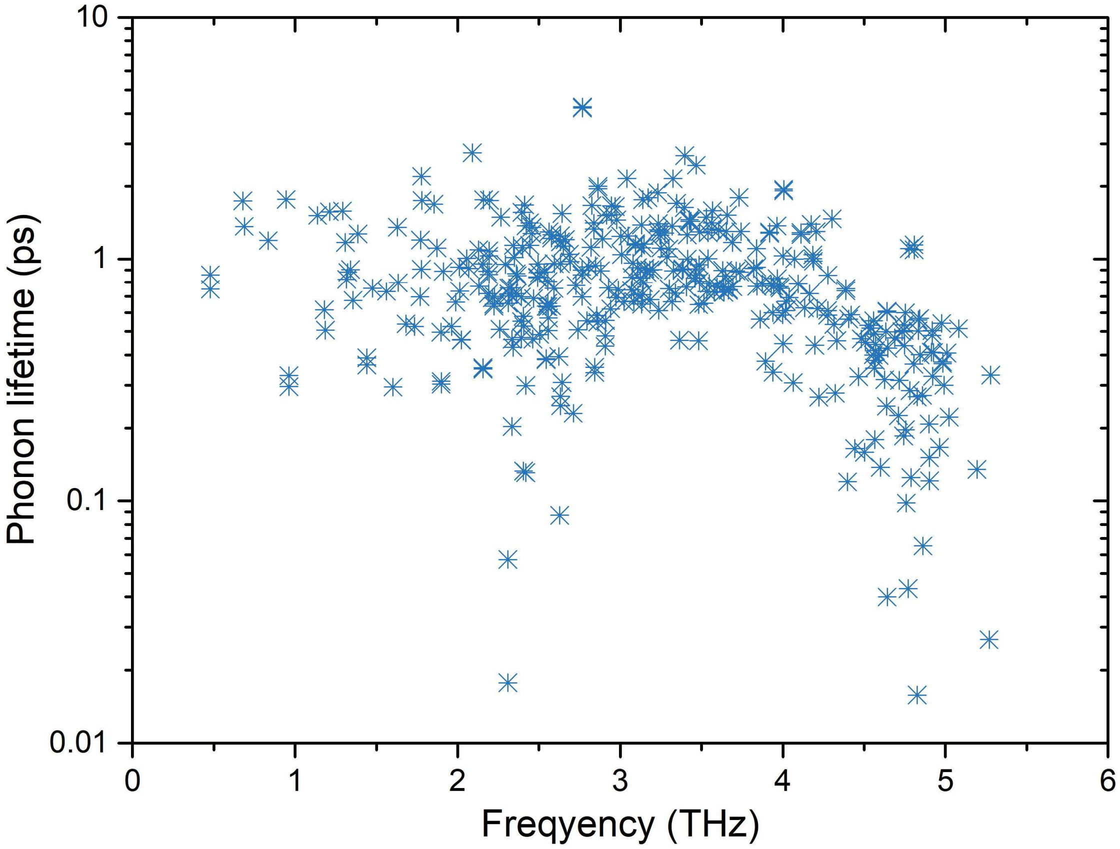


Fig.S9: The phonon lifetime of ε-iron at 330.68 GPa.

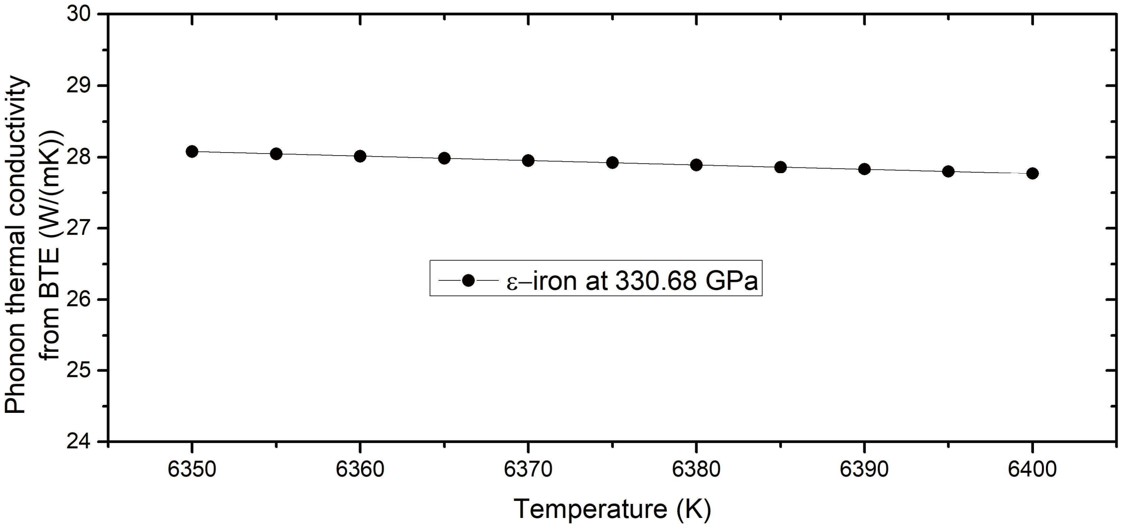


Fig.S10: The phonon (lattice) thermal conductivities ($\kappa_{ph}$) of the ε-iron at 330.68 GPa vs. temperature (6350 K- 6400 K) calculated from phonon BTE.

## 2.9 Analysis of propagation of errors

From the knowledge of the statistical average propagation of errors [19], we know that, when a variable is defined as $X = \frac{u}{v}$, the square of the error in $X$ can be expressed as

$$\sigma_X^2 = \sigma_{\frac{u}{v}}^2 = \sigma_u^2 \left(\frac{\partial X}{\partial u}\right)_{\bar{u}}^2 + \sigma_v^2 \left(\frac{\partial X}{\partial v}\right)_{\bar{v}}^2 = \frac{\sigma_u^2}{\bar{v}^2} + \frac{\sigma_v^2 \bar{u}^2}{\bar{v}^4}$$
$$\Rightarrow \left(\frac{\sigma_X}{\frac{\bar{u}}{\bar{v}}}\right)^2 = \left(\frac{\sigma_{\frac{u}{v}}}{\frac{\bar{u}}{\bar{v}}}\right)^2 = \left(\frac{\sigma_u}{\bar{u}}\right)^2 + \left(\frac{\sigma_v}{\bar{v}}\right)^2. \quad (9)$$

From Equation (19), we know that the error in $\kappa_{el}$ mainly originates from $\nabla T$ and $\frac{\partial \bar{U}_{EPO}(l)}{\partial N_l}$. As the $\nabla T$ calculation is based on the statistical time average of temperature of each single atom layer, the temperature fluctuation $\overline{(\Delta T)^2} = k_B T^2 / C_v$ [20] of each layer is large due to the small number of atoms in the layer. Thus, the conventional error estimate for $\nabla T$ is quite large. However, from Fig. S2 we find that the NEAIMD always yields a stable temperature profile after sufficient simulation time, and so we have reason enough to assume the linear fitting error as the error in $\nabla T$.

At the same time, we notice that the non-linear phenomenon of $\frac{\partial \bar{U}_{EPO}(l)}{\partial N_l}$, leads to a relatively large error in $\kappa_{el}$. We calculate the error in $\kappa_{el}$ (Table 4) from Equation (9). From Table 4 we can see that the $\kappa_{el}$ of ϵ-Fe have relatively large uncertainties, because of the large error in linear fit of $\nabla T$ and $\frac{\partial \bar{U}_{EPO}(l)}{\partial N_l}$.

Table 4. Error bar of electrical thermal conductivity $\kappa_{el}$ of ϵ-Fe at ~330 GPa, 6377 K.

| System | ϵ-Fe |
| --- | --- |
| Temperature (K) | 6377.06 |
| Pressure (GPa) | 330.68 |
| Error bar of linear fitting $\nabla T$ | 7.19% |
| Error bar of linear fitting $\frac{\partial \bar{U}_{EPO}(l)}{\partial N_l}$ | 6.24% |
| Total error bar of $\kappa_{el}$ (W/mK) | 8.50 |
| Total error bar of $\kappa_{el}$ (percentage) | 9.52% |

## References

[1] Kresse, G. & Furthmüller, J. Efficient iterative schemes for ab initio total-energy calculations using a plane-wave basis set. Phys. Rev. B **54**, 11169-11186 (1996).
[2] Kresse, G. & Furthmüller, J. Efficiency of ab-initio total energy calculations for metals and semiconductors using a plane-wave basis set. Comput. Mater. Sci. **6**, 15-50 (1996).
[3] Perdew, J. P., Burke, K. & Ernzerhof, M. Generalized Gradient Approximation Made Simple. Phys. Rev. Lett. **77**, 3865-3868 (1996).
[4] Blöchl, P. E. Projector augmented-wave method. Phys. Rev. B **50**, 17953-17979 (1994).
[5] Kresse, G. & Joubert, D. From ultrasoft pseudopotentials to the projector augmented-wave method. Phys. Rev. B. **59**, 1758-1775 (1999).
[6] Pozzo, M., Davies, C., Gubbins, D. and Alfè, D. Thermal and electrical conductivity of iron at Earth's core conditions. Nature **485**, 355 (2012).
[7] Pozzo, M., Davies, C., Gubbins, D. and Alfè, D. Thermal and electrical conductivity of solid iron and iron–silicon mixtures at Earth's coreconditions. Earth and Planetary Science Letters **393**, 159 (2014).
[8] de Wijs, G. A., Kresse, G., Vočadlo, L., Dobson, D., Alfè, D., Gillan, M. J., Price, G. D., The viscosity of liquid iron at the physical conditions of the Earth's core, Nature **392**, 805 (1998).
[9] Stackhouse, S., Stixrude, L. & Karki, B. B. Thermal Conductivity of Periclase (MgO) from First Principles. Phys. Rev. Lett. **104**, 208501 (2010).
[10] Yue, S.-Y., Zhang, X., Stackhouse, S., Qin, G., Di Napoli, E., Hu, M. Methodology for determining the electronic thermal conductivity of metals via direct non-equilibrium ab initio molecular dynamics, Phys. Rev. B **94**, 075149 (2016).
[11] Alfè, D. Ab initio molecular dynamics, a simple algorithm for charge extrapolation, Computer Physics Communications **118**, 31 (1999).
[12] Andersen, H. C., Molecular dynamics simulations at constant pressure and/or temperature, The Journal of Chemical Physics **72**, 2348 (1980).
[13] Müller-Plathe, F. A simple nonequilibrium molecular dynamics method for calculating the thermal conductivity. J. Chem. Phys. **106**, 6082-6085 (1997).
[14] Taylor, J. R. An Introduction to Error Analysis: The Study of Uncertainties in Physical Measurements (2nd Ed.). Ch.**4**, (University Science Books, 1997).
[15] Schelling, P. K., Phillpot, S. R. & Keblinski, P. Comparison of atomic-level simulation methods for computing thermal conductivity. Phys. Rev. B **65**, 144306 (2002).
[16] Togo, A., Oba, F. & Tanaka, I. First-principles calculations of the ferroelastic transition between rutile-type and $CaCl_2$-type $SiO_2$ at high pressures. Phys. Rev. B **78**, 134106 (2008).
[17] Li, W., Carrete, J., Katcho, N. A. & Mingo, N. ShengBTE: A solver of the Boltzmann transport equation for phonons. Comput. Phys. Commun. **185**, 1747-1758 (2014).
[18] Yue, S.-Y., Zhang, X., Qin, G., Phillpot, S. R., Hu, M., Metric for strong intrinsic fourth-order phonon anharmonicity. Phys. Rev. B **95**, 195203 (2017).
[19] Ku, H. H. Notes on the Use of Propagation of Error Formulas, Journal of Research of the National Bureau of Standards - C. Engineering and Instrumentation, **70C**, No.4 (1966).
[20] Landau, L. D. & Lifshitz, E. M. Statistical Physics, Part 1 (3rd Ed.) Ch.**2** (Pergamon Press, 1980).
